# Supplementary material for: Localization with Hopping Disorder in a Quasiperiodic Synthetic Momentum Lattice
Source: arXiv:2604.11855 source file (2026-10-01)
Supplement: Supplementary file 1 [file supp.tex]

\documentclass[pre,aps,amsmath,amssymb,superscriptaddress,notitlepage,twocolumn]{revtex4-2}

\usepackage{graphicx,multirow,outlines,ulem}
\usepackage{color}
\usepackage{hhline}
\usepackage{physics}
\usepackage{hyperref}
\usepackage{subcaption}

\usepackage{caption}
\usepackage{subcaption}
%\usepackage{lipsum}
%\captionsetup{skip=100pt}
\usepackage{float}
\usepackage{lipsum} % just for the example

\usepackage[mathscr]{eucal}
\captionsetup{%
    justification=Justified,%
}

\newcommand{\blu}{\color{blue}}

\usepackage{tikz}
\usepackage{xcolor}
\usepackage[section]{placeins}
\newcommand{\bo}{\begin{outline}}
\newcommand{\eo}{\end{outline}}

\newcommand{\qed}{\nobreak \ifvmode \relax \else
      \ifdim\lastskip<1.5em \hskip-\lastskip
      \hskip1.5em plus0em minus0.5em \fi \nobreak
      \vrule height0.75em width0.5em depth0.25em\fi}
%\flushbottom
\begin{document}
\title{%
  {\blu{Supplementary Information}} \\
  \large Localization with Hopping Disorder in Quasi-periodic Synthetic Momentum Lattice}

\maketitle

\section{State-Resolved Localization and Local Disorder Environment}

To clarify how spatial correlations in hopping disorder affect individual eigenstates, we introduce state-resolved measures that quantify the effective local disorder environment sampled by each eigenstate.  For eigenstate $|\psi_n\rangle = \sum_i \psi_n(i)\,|i\rangle$ with probability density $\rho_n(i) = |\psi_n(i)|^2$, we assign to each bond $(i,\,i{+}1)$ a weight proportional to the wavefunction's local occupation:

\begin{equation}
w_n(i) = \frac{\rho_n(i) + \rho_n(i+1)}{2}, \quad \sum_i w_n(i) = 1.
\label{eq:bond_weight}
\end{equation}

This bond-weight construction ensures that the resulting local measures probe only the spatial region that is effectively visited by $|\psi_n\rangle$, suppressing contributions from sites far from the wavefunction's support. We then define the \textit{local hopping mean} and \textit{local hopping variance} for eigenstate $n$ as
\begin{align}
  \langle t \rangle_{\mathrm{loc},n} &= \sum_i t_i\,w_n(i), \label{eq:tlocal}\\
  \sigma^2_{t,n} &= \sum_i \bigl(t_i - \langle t \rangle_{\mathrm{loc},n}\bigr)^2 w_n(i). \label{eq:varlocal}
\end{align}
The quantity $\langle t \rangle_{\mathrm{loc},n}$ characterizes the \textit{effective} tunneling strength experienced by state $n$, while $\sigma^2_{t,n}$ measures the roughness of the disorder landscape in its vicinity. Figure~\ref{fig:local_hopping} reveals a striking qualitative distinction between spatially correlated and uncorrelated hopping disorder. We quantify this relationship via the Pearson correlation coefficient

\begin{equation}
r = \frac{\text{Cov}(\text{IPR}, |\langle t\rangle_{\mathrm{loc}}|)}{\sqrt{\text{Var}(\text{IPR})\, \text{Var}(|\langle t\rangle_{\mathrm{loc}}|)}},
\label{eq:pearson}
\end{equation}
where $\text{Cov}(X,Y) = \langle XY \rangle - \langle X \rangle \langle Y \rangle$ and averages are over eigenstates in the spectral center.\\

\begin{figure}[t]
\centering
\includegraphics[width=\columnwidth]{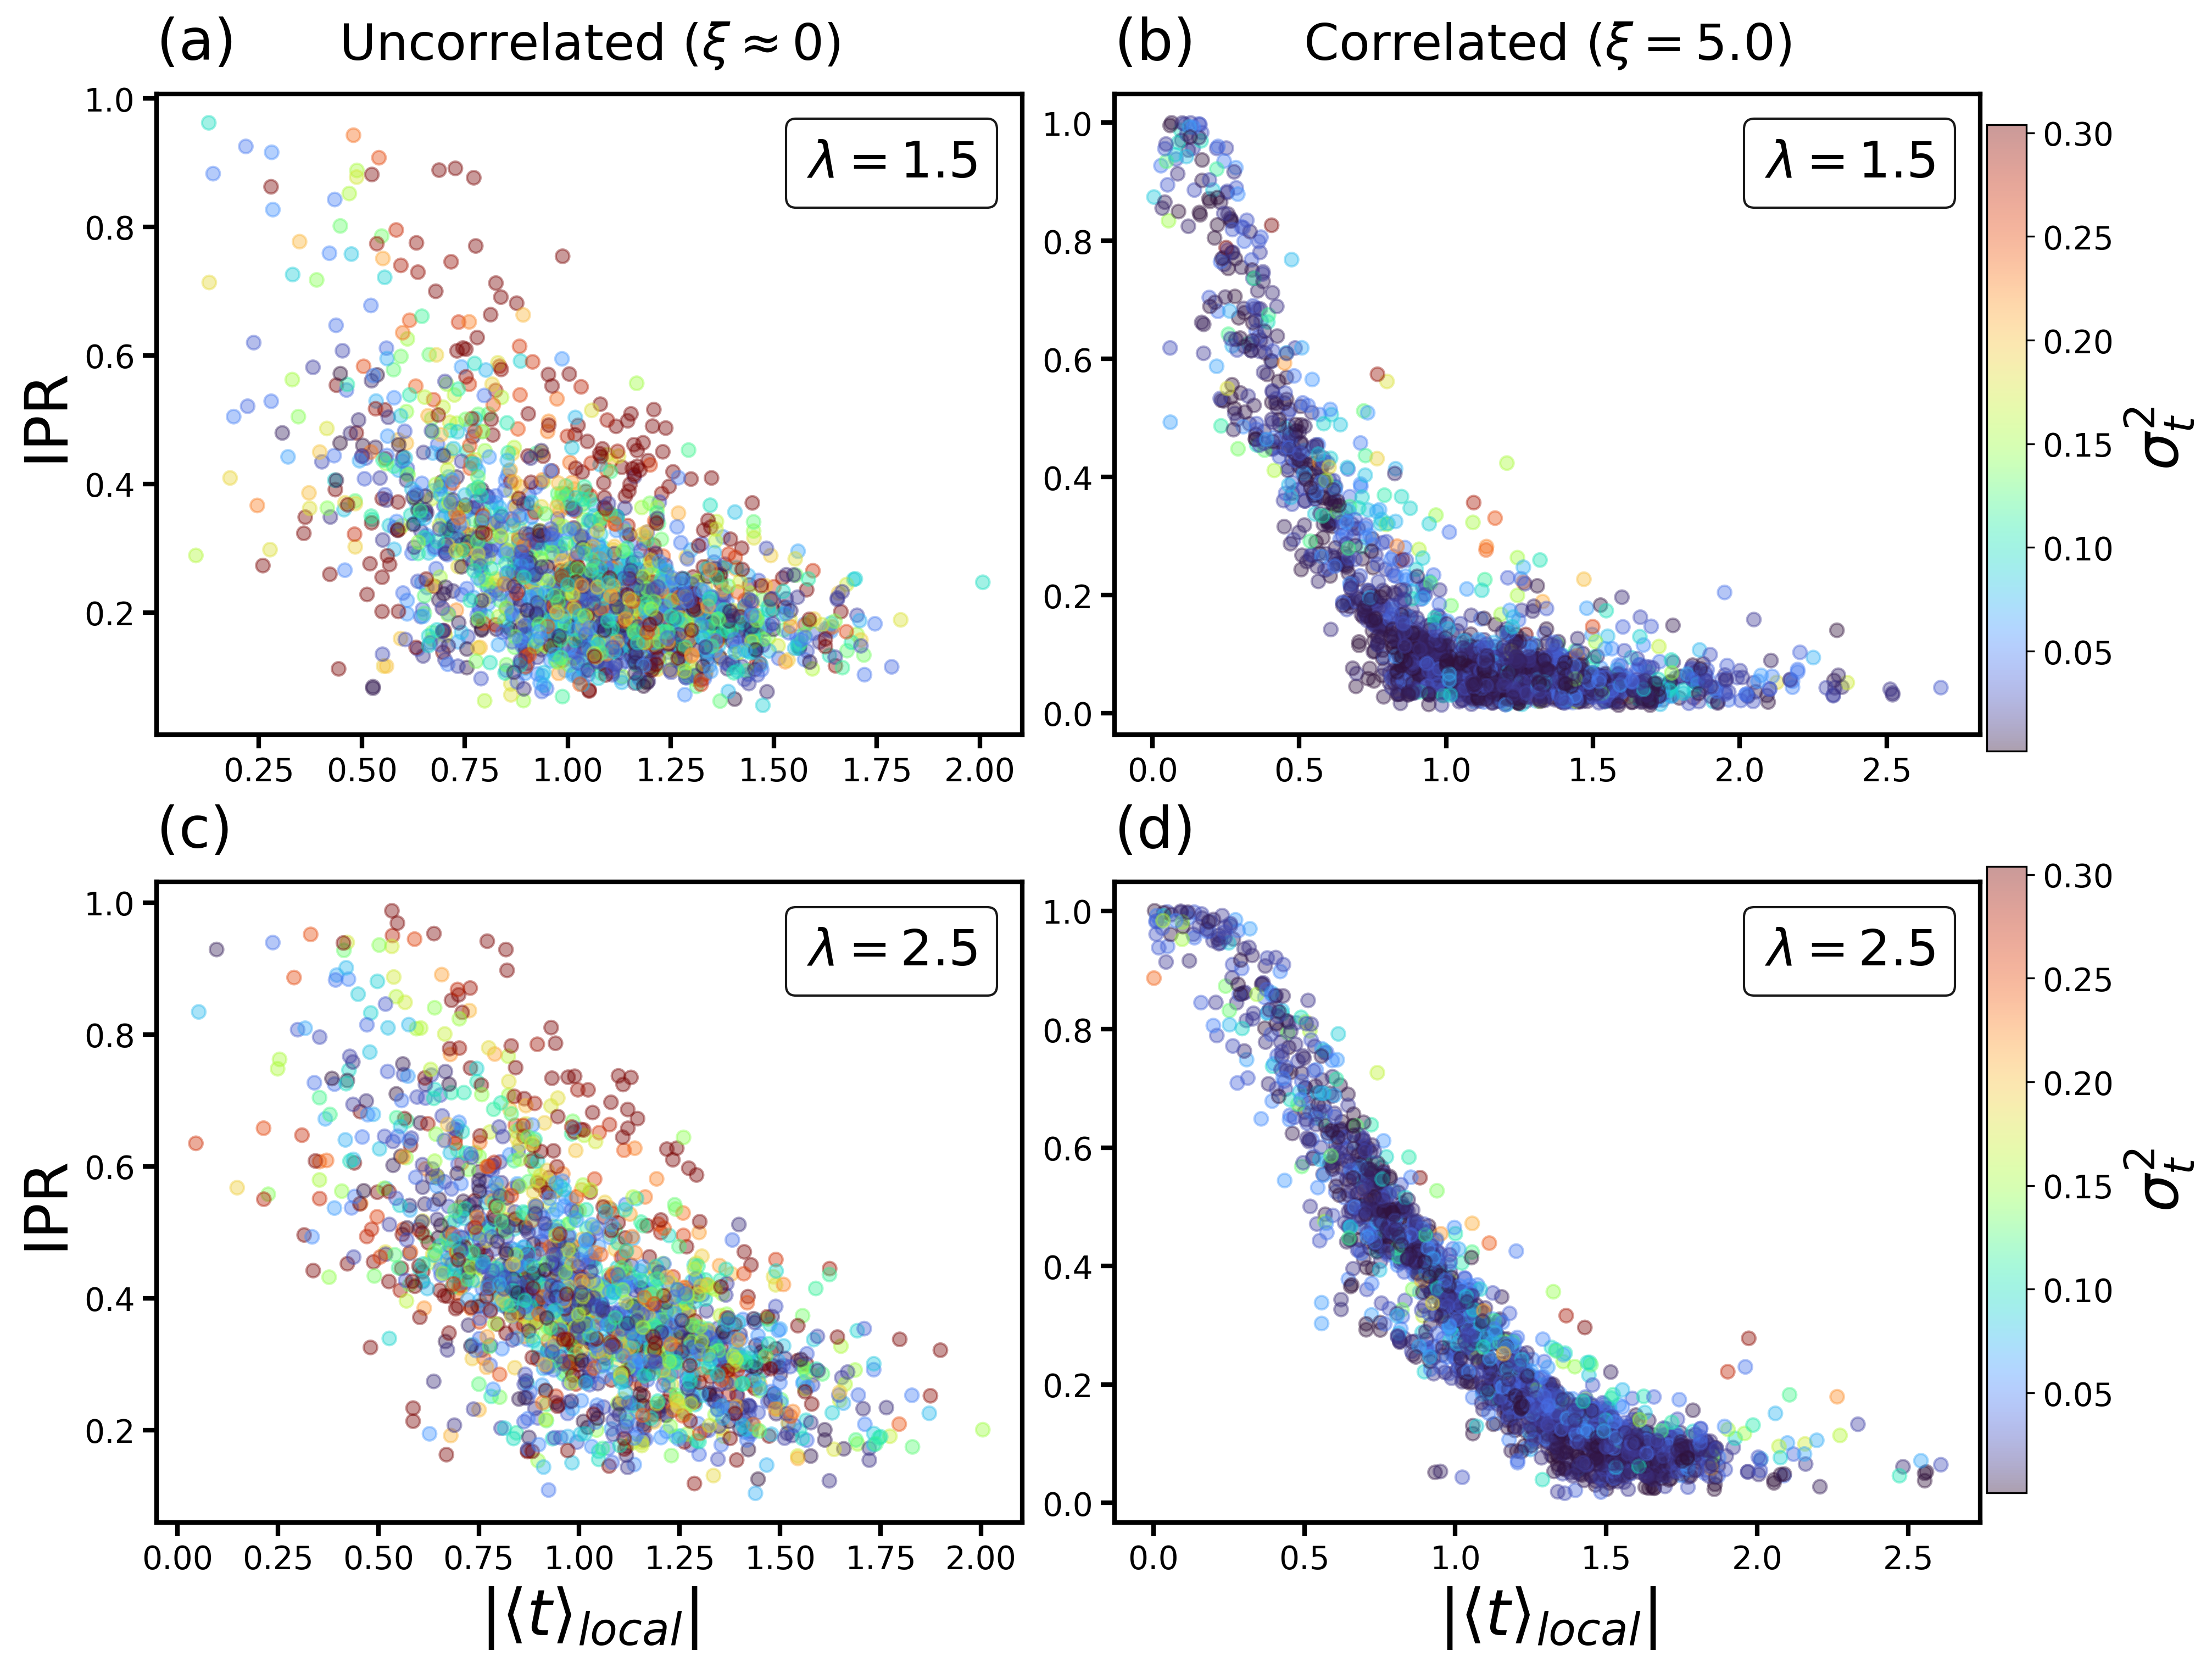}
\caption{(b,d) Correlated disorder: Eigenstates collapse onto narrow curve with strong anticorrelation ($r \simeq -0.96$), demonstrating that local hopping magnitude $|\langle t\rangle_{\mathrm{loc}}|$ nearly determines IPR. 
(a,c) Uncorrelated disorder: Broad scatter with weak correlation ($r \simeq -0.3$) indicates local mean is poor predictor when short-scale fluctuations dominate. Top/bottom: $\lambda=1.5/2.5$. Each point is one eigenstate; color encodes local variance $\sigma_t^2$ (comparable range in both cases).}
\label{fig:local_hopping}
\end{figure}

\paragraph{Correlated disorder}: Eigenstates collapse onto a narrow curve with extremely strong anticorrelation ($r \simeq -0.96$).  States residing in high-hopping regions ($\langle t \rangle_{\mathrm{loc}} > 1$) are systematically less localized, while those in low-hopping regions exhibit large IPR. This deterministic relationship persists across the AA transition ($\lambda=2$), with the functional form $\text{IPR}(\langle t \rangle_{\mathrm{loc}})$ preserved despite an overall upward shift in localization strength. The saturation of IPR at large $\langle t \rangle_{\mathrm{loc}}$ reflects geometric confinement: eigenstates cannot extend beyond the correlated region size $\xi$, yielding $\ell_{\mathrm{loc}} \sim \min(\xi, \ell_{\mathrm{AA}})$, where $\ell_{\mathrm{AA}}(\lambda)$ is the Aubry-Andr\'e localization length. 
Even in high-hopping regions, the quasiperiodic potential $V_i = \lambda \cos(2\pi\beta i)$ prevents full delocalization, producing quasi-extended states confined to finite transmission domains.\\

\paragraph{Uncorrelated disorder}
The scatter plot exhibits broad dispersion with weak anticorrelation ($r \simeq -0.3$). 
Although a negative trend persists on average, individual eigenstates at a given $\langle t \rangle_{\mathrm{loc}}$ show widely varying IPR values. This indicates that local hopping magnitude is a poor predictor of localization when bond-to-bond fluctuations induce strong random backscattering. Isolated high-hopping bonds cannot support coherent transport, as they are embedded in a fluctuating environment with high local variance $\sigma_t^2$.
Crucially, the local hopping variance $\sigma_t^2$ has comparable magnitude in both cases due to normalization. The qualitative difference arises from spatial organization: correlated disorder redistributes variance into smooth regions supporting locally enhanced transport, whereas uncorrelated disorder concentrates variance into short-scale fluctuations that suppress transport.\\

\section{Experimental Setup}
\label{sec:expt}

The experiment begins by loading $^{87}$Rb atoms from a Zeeman slower into a Magneto-Optical Trap (MOT), where they are laser-cooled to $\sim 50\,\mu\mathrm{K}$. The pre-cooled atoms are then transferred into a Crossed Dipole Trap (XDT) formed by two tightly focused, counter-propagating $1064\,\mathrm{nm}$ beams. Forced evaporative cooling
in the XDT reduces the temperature to $\sim 50\,\mathrm{nK}$, producing a Bose-Einstein
Condensate (BEC) of approximately $4\times10^4$ atoms.\\

For creating the lattice we use two 1064 nm beams travelling opposite to each other which is aligned with the condensate. The schematic of our optical setup is given below. We use two Acousto-Optic Modulators (AOMs) to address the different Bragg transitions \cite{stenger1999bragg}. We can create a lattice of momentum states with momentum steps of $2\hbar k$, $p=...-2\hbar k, 0, 2\hbar k... $, where $k$ is the wavevector of our 1064 nm beam. The kinetic energy of each state is given by $E=\frac{p^{2}}{2m}$, so the energy difference between each state is unique. We need a separate tone for each transition \cite{meier2016msl}. For this, We drive one of our two AOMs with a multi-tone signal. This allows us to independently control the amplitude, phase and energy detuning of each Bragg transition. It can be mapped to any one-dimensional tight-binding Hamiltonian and used to simulate it as explained in \cite{meier2016msl}.\newline

For generating the multi-tone we use a Spectrum AWG M4i.6631 that has a multi-tone DDS option. With this option the output of 20 DDS cores is combined into a single channel and sent to our Acousto-Optic Modulator through an amplifier. We randomize the phases of the tones to get a smoother output.  This also allows us to input more power without saturating the amplifier. 
We typically work with 1 ms pulses to drive the Bragg transitions. Beyond this the different momentum states are no longer spatially overlapped which leads to loss of coherence. We apply the pulse immediately after the dipole trap beams are switched off. We get best results without any time delay between when the dipole beams are switched off and lattice beams are switched on. We then let the different momentum states separate for 10 ms before absorption imaging to measure the population at each site. \newline
\textbf{Simulations of the momentum space lattice}: We perform numerical simulations of the ideal tight-binding model as well as a more complete simulation of the BEC dynamics in the momentum space lattice. The simulation of the BEC dynamics takes into account the momentum width of the BEC, off-resonant excitations of the lattice beams, and loss of coherence due to the momentum states splitting apart. The Hamiltonian is given by:
\begin{equation}
    \hat{H}(x)=\left(\frac{\hbar}{2m}\frac{\partial }{\partial x}\right)^{2} +\sum_{i=\frac{n}{2}}^{\frac{n}{2}-1}\Omega_{i} cos(2k_{o}x)cos(\omega_{i}t)
    \label{Eq: Simulation Hamiltonian}
\end{equation}
where, $\Omega_{i}$ is the Rabi frequency. n is the number of tones (which in our case is 20) and $\omega_i=4E_{r}(2i+1)$ is the resonant frequency between site $i$ and $i+1$. We use the split-operator method which is detailed in \cite{fleck1978gpe}. The evolution operator $\hat{U}(\Delta t)=exp[-i\hat{H}\Delta t/\hbar]$ is split into momentum and position space components---$\hat{U}_p(\Delta t)$ and $\hat{U}_{x}(\Delta t)$. Where, $\hat{U}_p(\Delta t)=exp[-ip^2\Delta t/2m\hbar]$ and $\hat{U}_x(\Delta t)=exp[-iV(x,t) \Delta t/\hbar]$. From Eq. \ref{Eq: Simulation Hamiltonian}, we get $V(x,t)=\sum_{i=\frac{n}{2}}^{\frac{n}{2}-1}\Omega_{i} cos(2k_{o}x)cos(\omega_{i}t)$ for the Momentum Space Lattice(MSL). Using Strang splitting the evolution operator can be decomposed as:
\begin{equation}
    \hat{U}(\Delta t)=\hat{U}_p(\Delta t/2)\hat{U}_x(\Delta t)\hat{U}_p(\Delta t/2)+O((\Delta t)^3)
\end{equation}
The second term quantifies the error from this decomposition. For an evolution of n steps of $\Delta t$ the evolution operator becomes:
\begin{multline}
    \hat{U}(n\Delta t)=\hat{U}_p(\Delta t/2)\hat{U}_x(\Delta t)\left(\prod_{n-1}\hat{U}_p(\Delta t)\hat{U}_x(\Delta t)\right)\\ \times\hat{U}_p(\Delta t/2)+O((\Delta t)^3)
\end{multline}
The wavevector is transformed back and forth between the position and momentum space using the Discrete Fourier Transform (DFT) and the respective evolution operators in each space are applied sequentially.\\ 
We take experimental data for the Rabi-oscillations between the 0th and 1st site. We can then approximately calculate the momentum width of the BEC by fitting the damped Rabi oscillations. We get a momentum width of $\Delta p=0.07\hbar k$. So we initialize the BEC as a Gaussian with momentum width $\Delta p=0.07\hbar k$ for all simulations of the GAA model.\\

\begin{figure*}
    \centering
    \includegraphics[width=0.9\linewidth]{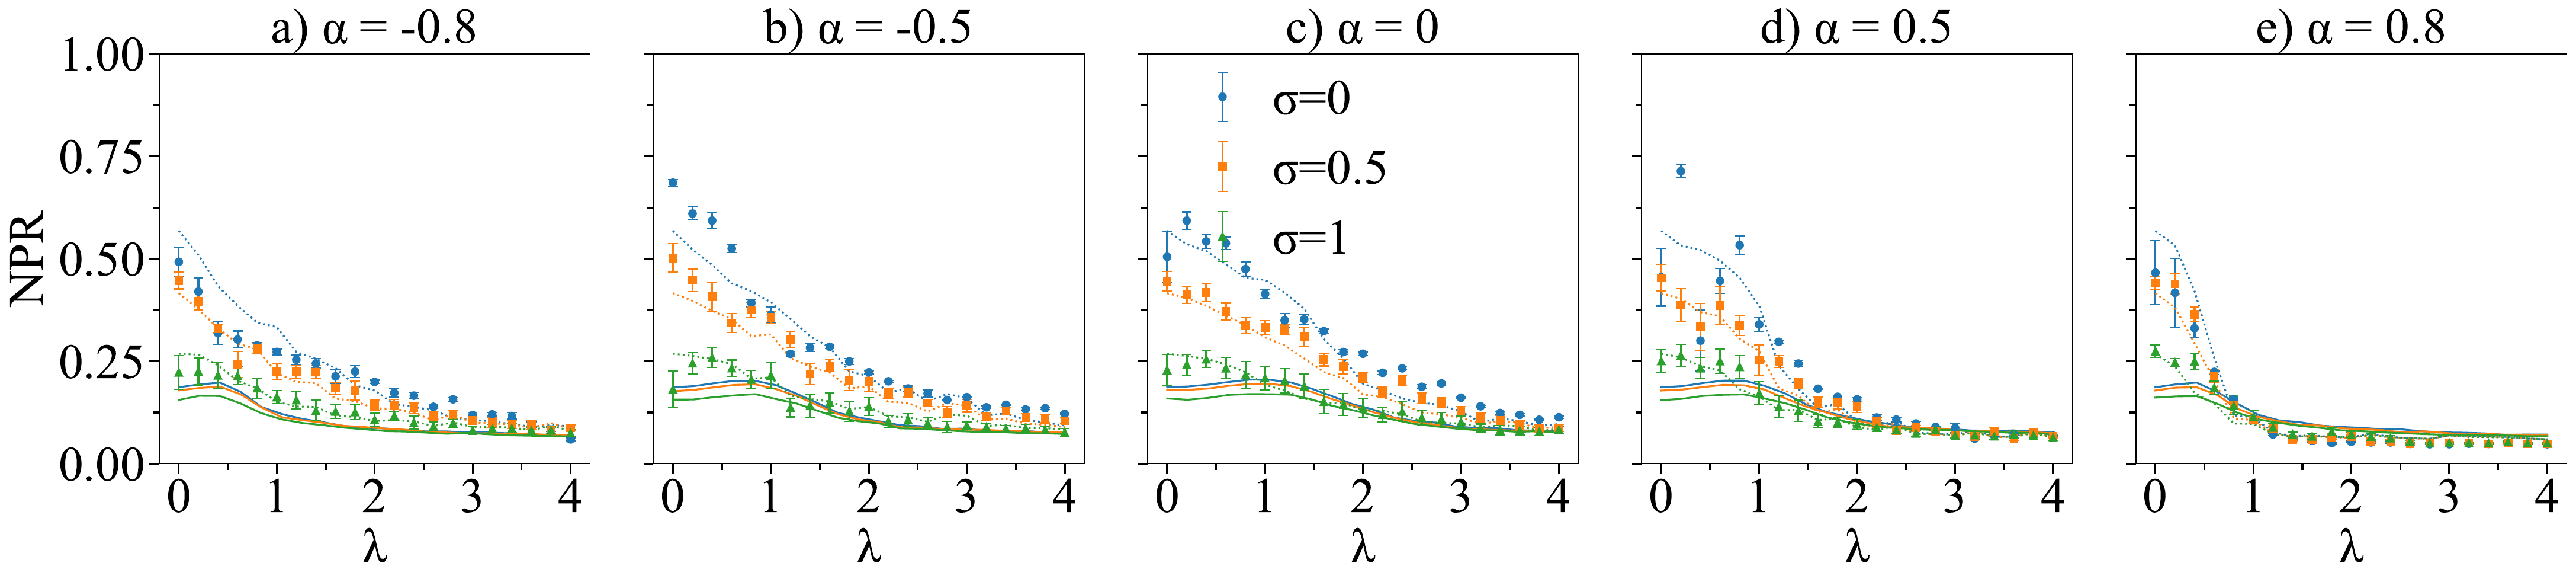}
    \caption{The NPR vs lambda plots for the GAA model. The NPR gives a clearer picture of the effect of adding disorder at smaller $\lambda$ values than the IPR.}
    \label{fig:NPR_all_alphas}
\end{figure*}

The normalized participation ratio (NPR) is defined as
\begin{equation}
  \mathrm{NPR}(\lambda) = \frac{1}{L\,\mathrm{IPR}(\lambda)},
  \label{eq:npr}
\end{equation}
where $L$ is the system size. An NPR of order unity indicates a state spread across the full lattice, whereas NPR$\,\sim\chi/L$ signals a state localized over $\chi$ sites. Figure~\ref{fig:NPR_all_alphas} shows the NPR as a function of $\lambda$ for all five values of $\alpha$ and three disorder strengths. Importantly, upon introducing disorder, the effect of localization becomes clearly visible in the NPR even at small $\lambda$, where the IPR remains close to zero and exhibits only weak variation across disorder strengths. \\

\bibliography{ref}

\end{document}
